# Supplementary material for: I3DE: An IDE for Inspecting Inconsistencies in PL/SQL Code
Source: arXiv:2403.03433 source file (2024-03-06)
Supplement: Supplementary file 1 [file 7_Appendix.tex]

%%
%% If your work has an appendix, this is the place to put it.
\appendix

\section{User Study Tasks}\label{sec:user-study-tasks}

\subsection{Inconsistency by Presumption}
\begin{figure}[H]
\lstset{
 tabsize=2,
 basicstyle=\tt\scriptsize,
 columns=fixed,       
 numbers=left,
 numbersep=4pt,
 numberstyle=\tiny\color{darkgray},
 frame=none,
 backgroundcolor=\color[RGB]{245,245,245},
 keywordstyle=\bfseries,
 commentstyle=\it\color[RGB]{0,96,96},
 showstringspaces=false,
 language=SQL,
 morekeywords={FUNCTION, DECLARE, IF, ELSIF, RETURN, FOR, LOOP, LANGUAGE, RETURNS, VOID, AS},
}
\begin{lstlisting}[]
-- Fill in the blank of the procedure.
-- Consider an information system in which identity privileges are
-- assigned according to the first character of the account number,
-- with 1 being the supervisor.
-- The following procedure determines whether a user is a
-- non-supervisor by passing in the user's account number
-- and, if so, issues an alert.
CREATE FUNCTION giveAlert(account CHAR) RETURNS boolean AS $$
BEGIN
  IF _____ != '1' THEN              -- fallacy: account
    raise notice 'GIve an alert!';  -- correct: account::CHAR
    RETURN true;
  ELSE
    RETURN false;
  END IF;
END;
$$ LANGUAGE plpgsql;
\end{lstlisting}
% \vspace{-9pt}
\caption{User study task designed on inconsistency by presumption.}
\label{fig:presumption_task}
% \vspace{-9pt}
\end{figure} 

\subsection{Inconsistency by Overlook}
\input{sections/7_Appendix_Figure_Overlook}

\subsection{Inconsistency by Equivocality}
\begin{figure}[H]
\lstset{
 tabsize=2,
 basicstyle=\tt\scriptsize,
 columns=fixed,       
 numbers=left,
 numbersep=4pt,
 numberstyle=\tiny\color{darkgray},
 frame=none,
 backgroundcolor=\color[RGB]{245,245,245},
 keywordstyle=\bfseries,
 commentstyle=\it\color[RGB]{0,96,96},
 showstringspaces=false,
 language=SQL,
 morekeywords={FUNCTION, DECLARE, IF, ELSIF, RETURN, FOR, LOOP, LANGUAGE, RETURNS, VOID, AS},
}
\begin{lstlisting}[]
-- Indicate the result of running the procedure.
-- There's a table tb_employee(col_id, col_salary) in current DBMS.
-- col_id, col_salary are INT type.
-- Now expect the col_salary column to be written to the new table
-- salary_backup.
CREATE OR REPLACE FUNCTION backupSalary() RETURNS void AS $$
BEGIN
  SELECT col_salary INTO tsalary_backup FROM tb_employee;
END;                 -- fallacy: treat tsalary_backup as a table
$$ LANGUAGE plpgsql; -- correct: treat tsalary_backup as a variable
\end{lstlisting}
% \vspace{-9pt}
\caption{User study task designed on inconsistency by equivocality.}
\label{fig:equivocality_task}
% \vspace{-9pt}
\end{figure} 

\section{Answers by Generative Language Model}\label{sec:gen-model}
\noindent\textbf{User:} Please fill in the PL/pgSQL code blanks below: [Task 2 Code]\\
\noindent\textbf{ChatGPT3.5:} {\ttfamily total\_num * percentage}\\
\noindent\textbf{User:} Does your answer make the PL/pgSQL code inconsistent in any way?\\
\noindent\textbf{ChatGPT3.5:} {\ttfamily ROUND(total\_num * percentage)}\\
\noindent\textbf{User:} Is it appropriate to use {\ttfamily ROUND}?\\
\noindent\textbf{ChatGPT3.5:} {\ttfamily CEIL}, {\ttfamily FLOOR} or {\ttfamily ROUND}\\

\noindent\textbf{User:} Please fill in the PL/pgSQL code blanks below: [Task 2 Code]\\
\noindent\textbf{ChatGPT4:} {\ttfamily ROUND(total\_num * percentage)}\\
\noindent\textbf{User:} Is it appropriate to use {\ttfamily ROUND}?\\
\noindent\textbf{ChatGPT4:} {\ttfamily CEIL}, {\ttfamily FLOOR} or {\ttfamily ROUND}\\
