# Supplementary material for: I3DE: An IDE for Inspecting Inconsistencies in PL/SQL Code
Source: arXiv:2403.03433 source file (2024-03-06)
Supplement: Supplementary file 2 [file 7_Appendix_Figure_Equivocality.tex]

\begin{figure}[H]
\lstset{
 tabsize=2,
 basicstyle=\tt\scriptsize,
 columns=fixed,       
 numbers=left,
 numbersep=4pt,
 numberstyle=\tiny\color{darkgray},
 frame=none,
 backgroundcolor=\color[RGB]{245,245,245},
 keywordstyle=\bfseries,
 commentstyle=\it\color[RGB]{0,96,96},
 showstringspaces=false,
 language=SQL,
 morekeywords={FUNCTION, DECLARE, IF, ELSIF, RETURN, FOR, LOOP, LANGUAGE, RETURNS, VOID, AS},
}
\begin{lstlisting}[]
-- Indicate the result of running the procedure.
-- There's a table tb_employee(col_id, col_salary) in current DBMS.
-- col_id, col_salary are INT type.
-- Now expect the col_salary column to be written to the new table
-- salary_backup.
CREATE OR REPLACE FUNCTION backupSalary() RETURNS void AS $$
BEGIN
  SELECT col_salary INTO tsalary_backup FROM tb_employee;
END;                 -- fallacy: treat tsalary_backup as a table
$$ LANGUAGE plpgsql; -- correct: treat tsalary_backup as a variable
\end{lstlisting}
% \vspace{-9pt}
\caption{User study task designed on inconsistency by equivocality.}
\label{fig:equivocality_task}
% \vspace{-9pt}
\end{figure}
